# Supplementary material for: Improving robustness against common corruptions by covariate shift adaptation
Source: arXiv:2006.16971 source file (2020-10-23)
Supplement: Supplementary file 1 [file fixup_hyperparameters.tex]

\begin{table}[htp]\footnotesize
    \begin{minipage}{.5\linewidth}
      \centering
      \setlength{\tabcolsep}{5pt}
    \captionsetup{width=.95\textwidth}
    \caption{Hyperparameters for training the Fixup models.}
    \small
\begin{tabular}{ll}
    \toprule
    Parameter & Value \\
    \midrule
    optimizer & SGD-M \\
    learning rate & 0.1 \\
    momentum & 0.9 \\
    batch size & 256 \\
    epochs & 100 \\
    weight decay & \num{1e-4} \\
   \bottomrule
\end{tabular}
          \label{tbl:fixup_hyper}
    \end{minipage}%
    \begin{minipage}{.5\linewidth}
      \centering
\setlength{\tabcolsep}{5pt}
     \captionsetup{width=.75\textwidth}
    \caption{Hyperparameters for training the Groupnorm models.}
    \small
\begin{tabular}{ll}
   \toprule
     Parameter & Value \\
    \midrule
    optimizer & SGD-M \\
    learning rate & 0.1\\
    momentum & 0.9 \\
    batch size & 256 \\
    epochs & 100 \\
    weight decay & \num{1e-4} \\
   \bottomrule
\end{tabular}
      \label{tbl:group_norm_hyper}
    \end{minipage} 
\end{table}
