# Supplementary material for: Improving robustness against common corruptions by covariate shift adaptation
Source: arXiv:2006.16971 source file (2020-10-23)
Supplement: Supplementary file 2 [file objnet_mapping.tex]

\newpage
\subsection{Mapping of ambiguous classes in ON to IN}
\label{app:objnet-mapping}

There are nine classes in ON that have multiple possible mappings to IN. We have discarded these classes in our evaluation. Out of the proposed 113 classes in ON that overlap with IN according to the ON publication, we therefore only test on 104 classes. The ambiguous classes and possible mappings are given in Table~\ref{ON:ambiguous}. 

\begin{table}[ht]
    \centering
    \small
    \begin{tabular}{l l }
         \toprule
           \\
          ObjN class & IN classes \\
         \midrule
         wheel & wheel; paddlewheel, paddle wheel \\
         helmet & football helmet; crash helmet \\
         chair & barber chair; folding chair; rocking chair, rocker \\
         still\_camera & Polaroid camera, Polaroid Land camera; reflex camera \\
         alarm\_clock & analog clock; digital clock \\
         tie & bow tie, bow-tie, bowtie; Windsor tie \\
         pen & ballpoint, ballpoint pen, ballpen, Biro; quill, quill pen; fountain pen  \\
         bicycle & mountain bike, all-terrain bike, off-roader; bicycle-built-for-two, tandem bicycle, tandem \\
         skirt & hoopskirt, crinoline; miniskirt, mini; overskirt \\
    \end{tabular}
    \caption{Mapping between 9 ambiguous ON classes and the possible correspondences in IN. Different IN classes are separated with a semicolon.
    }
        \label{ON:ambiguous}
\end{table}
